# Supplementary material for: PEARLS: Near Infrared Photometry in the JWST North Ecliptic Pole Time Domain Field
Source: arXiv:2309.00031 ancillary file (2023-09-05)
Supplement: Supplementary file 1 [file NEP_MMIRS_HSC_data_release.pdf]

## PEARLS : The North Ecliptic Pole Time Domain Field: MMT/MMIRS and Subaru/HSC data

CHRISTOPHER N. A. WILLMER,<sup>1</sup> SETH H. COHEN,<sup>2</sup> ROLF A. JANSEN,<sup>2</sup> SATOSHI KIKUTA,<sup>3</sup> ROGIER A. WINDHORST,<sup>2</sup> AND MARIO NONINO<sup>4</sup>

<sup>1</sup>*Steward Observatory, University of Arizona, 933 North Cherry Avenue, Tucson, AZ 85721, USA*

<sup>2</sup>*School of Earth & Space Exploration, Arizona State University, 550 E. Tyler Mall, Tempe, AZ 85287-1404, USA*

<sup>3</sup>*National Astronomical Observatory of Japan, 2-21-1 Osawa, Mitaka, Tokyo 181-8588, Japan*

<sup>4</sup>*INAF-Trieste Astronomical Observatory, Via Bazzoni 2, IT-34124, Trieste, Italy*

(Dated: Wednesday 30<sup>th</sup> August, 2023)

### 1. ABSTRACT

We make available catalogues and image mosaics of the JWST North Ecliptic Pole Time Domain Field in the visible and near infrared. These mosaics come from observations in  $Y$ ,  $J$ ,  $H$  and  $K$  obtained with the MMT-Magellan Infrared Imager and Spectrometer (MMIRS) on the MMT and from archival images in  $g$ ,  $i2$ ,  $NB816$ ,  $z$  and  $NB921$  of the Hyper-Suprime-Cam (HSC) obtained with the Subaru telescope. These images are astrometrically calibrated in the GAIA DR3 (MMIRS) and GAIA DR1 (HSC) systems with position dispersions  $\leq 70$  milliarcseconds (mas) for MMIRS and  $\leq 20$  mas for HSC data. The joint visible-NIR catalogue contains over 57,000 sources and was used to estimate depths attained by these images. We find that the AB magnitudes of point sources with  $1\sigma$  above the background using single band detections at a 95% completeness level are ( $g$ ,  $i2$ ,  $z$ ,  $NB816$ ,  $NB921$ ,  $Y$ ,  $J$ ,  $H$ ,  $K$ ) = (25.68, 24.50, 24.09, 23.96, 24.08, 23.80, 23.53, 23.13, 23.28).

### 2. OVERVIEW

The JWST North Ecliptic Pole Time Domain Field (NEP TDF) has been targeted since 2016 by a variety of observatories from the ground and from space to identify and characterise transient sources and provide baseline data for observations from space before the launch of JWST. This data release makes available reduced image mosaics and catalogues derived from observations with the MMT-Magellan Infrared Imager and Spectrometer (MMIRS) on the MMT and from archival images of the Hyper-Suprime-Cam obtained in 2017 with the Subaru telescope in visible/NIR wavelengths as part of the Hawaii EROSita Ecliptic pole Survey (HEROES; e.g., Songaila et al. 2018, Taylor et al. 2023). The observations, reduction, mosaic making and catalogue preparation are described in Willmer et al. (2023) hereafter Paper1. Here we present additional details on the astrometric and photometric calibrations of the images and gives a brief description of the derived catalogue. All magnitudes are quoted in the AB system (Oke & Gunn 1983) and, following Willmer (2018), we adopt the Vega to AB transformations ( $MMIRS-Y$ ,  $MMIRS-J$ ,  $MMIRS-H$ ,  $MMIRS-K$ ,  $MMIRS-K_{\text{spec}}$ ) = (0.574, 0.891, 1.333, 1.836, 1.840) mag. In this document we will use a shorthand for filter names being referred as  $g$ ,  $i2$ ,  $z$ ,  $Y$ ,  $J$ ,  $H$ ,  $K$  and  $K_{\text{spec}}$  excepting in the case of the  $HSC-Y$  filter so there is no ambiguity.

### 3. MMIRS DATA

In the next two sections, we give a brief overview of the data reduction (described in detail in Paper1), and assess the calibrations. The MMIRS data were reduced using a sequence of IDL scripts and custom written software. The initial steps require converting the raw data cubes into images with count rates in data numbers per second (DN/s), and used the Chilingarian et al. (2015) IDL procedures<sup>1</sup>, with a few adaptations for use with imaging data that are

<sup>1</sup> [https://bitbucket.org/chil\\_sai/mmirs-pipeline/wiki/Home](https://bitbucket.org/chil_sai/mmirs-pipeline/wiki/Home)

publicly available at [https://github.com/cnaw/mmirs\\_imaging](https://github.com/cnaw/mmirs_imaging). The count-rate images go through 2 iterations of sky-subtraction, the first using a mask calculated by the MMIRS team that flags bad pixels, the second masking bad pixels and detected sources. In the first iteration the sky-subtracted images are analysed with **SExtractor** (Bertin & Arnouts 1996) to identify stars, which are used for the initial astrometric calibration and to estimate each image’s seeing FWHM. These images are also used to identify saturated sources and bogus sources due to latent charges. The sources and bad pixels are used to create masks used in the second sky-subtraction iteration, which are derived from the segmentation image created by **SExtractor**. In these masks the outline of each detected object is extended radially by 2 pixels to remove light from the outer regions of sources, while in the case of objects due to persistence, the outline is extended by 5 pixels because of their flatter profile. After the second round of sky-subtraction, the images are astrometrically calibrated using the **astrometry.net** software of Lang et al. (2010) with the Gaia DR3 catalogue (Gaia Collaboration 2022) as reference. The astrometric solutions have typical RMS residuals of  $\sim 0''.03$  per image.

Creating the mosaics involves: (1) using **scamp** (Bertin 2011) to calculate an astrometric solution compatible with **swarp**; (2) finding the photometric offsets between individual images, using the first image in a list as reference; (3) using **swarp** to calculate the mosaics proper. The final mosaics were centered at the same position (17:22:48.1298, +65:50:14.853, J2000) as the HSC images described below and using the same pixel size of  $0''.168$ . These images contain  $11,000 \times 12,000$  pixels. The photometric calibration of the mosaics followed Almeida-Fernandes et al. (2022) using GAIA EDR3 stars with measurements in SDSS (Abdurro’uf et al. 2022), Pan-STARRS (Tonry et al. 2012), and 2MASS (Skutskie et al. 2003, 2006) and the stellar models of Coelho (2014). As described in Paper1, there are three modalities of  $K$ -band data ( $K_{0.95}$ ,  $K_{2.68}$ ,  $K_{\text{spec}}$ ) with slightly different zero-points. Using objects in common, the final values of  $K$  fluxes and magnitudes were calculated by multiplying/adding offsets, and, when more than one measurement is available, using an inverse variance weighted average.

The astrometric quality of the mosaics was assessed using the GAIA DR3 catalogue and the comparison is presented in Figures 1 through 4 with the results shown in Table 1. The number of GAIA stars contained within the footprints is slightly less than 400 for  $Y$ ,  $H$ ,  $K$  and 485 stars for  $J$ ; the average offsets are of  $\lesssim 35$  milli-arcseconds (mas) and the dispersions of  $\lesssim 70$  mas for the NIR imaging. The figures clearly show that there are small-scale distortions of  $\lesssim 0''.15$  remaining in the NIR data with a few poles within the field of view. The cause of these distortions is currently unknown.

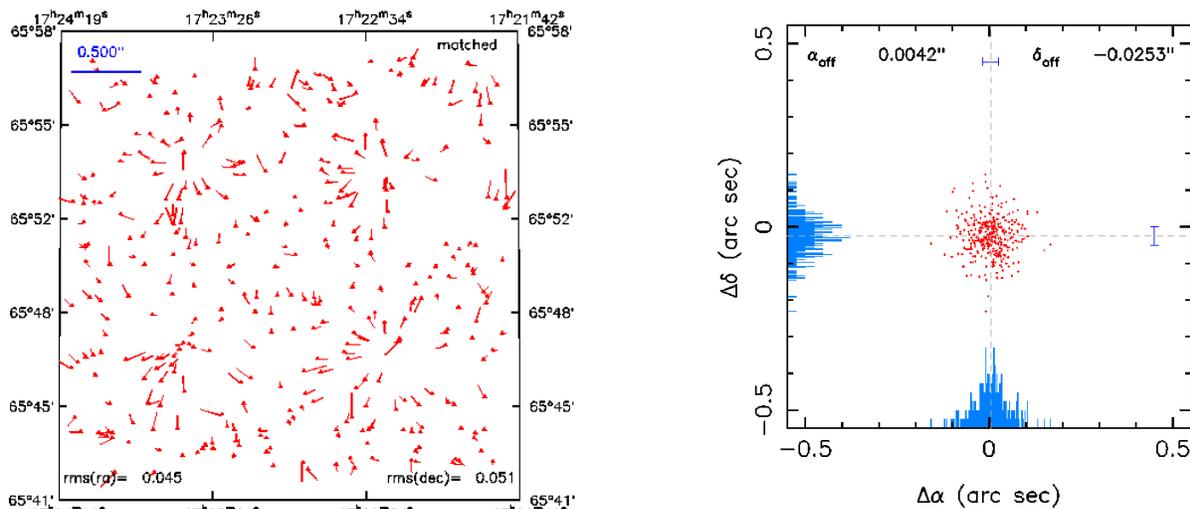

**Figure 1.** Comparison between sources detected in the  $Y$  mosaic and GAIA DR3 stars. The left panel shows the vector differences between positions, with a scale ledger line in the upper left corner showing the search radius of  $0''.50$ . The values in the bottom show the dispersion in arcseconds of the mean position differences in Right Ascension (R.A.) and Declination (Dec.). The right panel shows the distribution of position differences. The values on top denote the mean offsets in R.A. and Dec. in arcseconds.

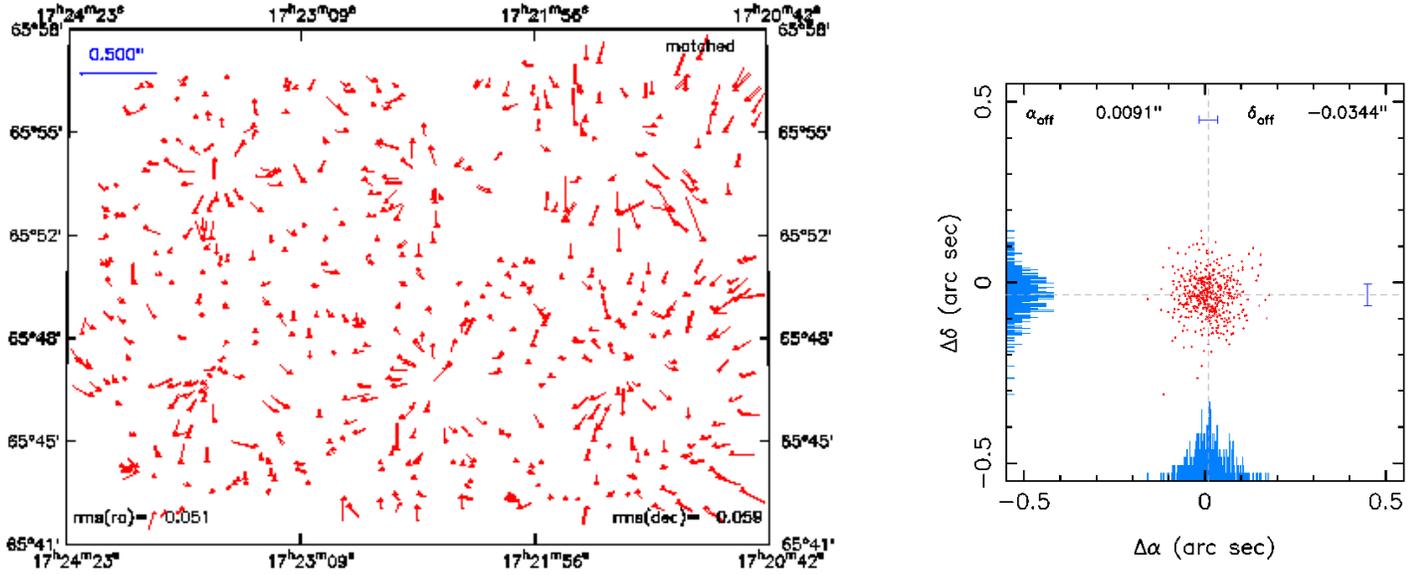

Figure 2. Same as in Figure 1 for the *J* band.

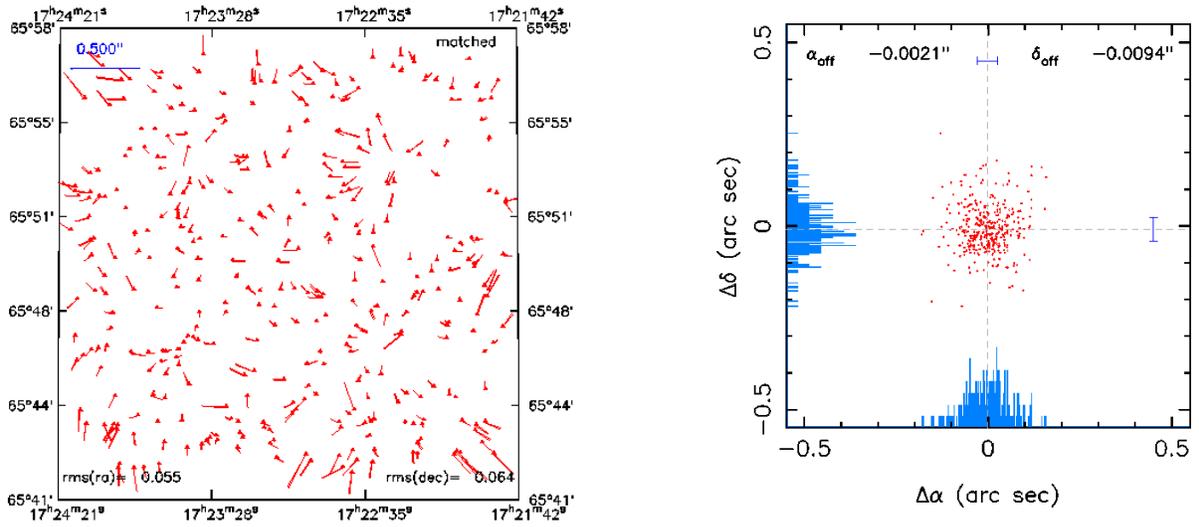

Figure 3. Same as in Figure 1 for the *H* band.

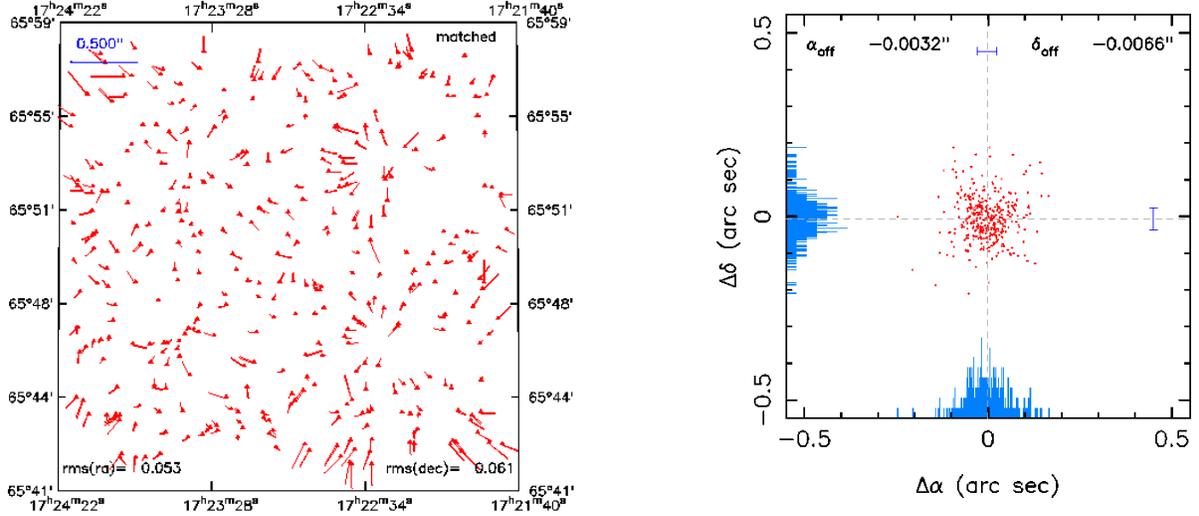

**Figure 4.** Same as in Figure 1 for the K band.

**Table 1.** Comparison between positions measured on the mosaics with the GAIA DR3 catalogue

| Filter  | mean( $RA_{GAIA}-RA$ ) | $\sigma(RA_{GAIA}-RA)$ | mean( $Dec_{GAIA}-Dec$ ) | $\sigma(Dec_{GAIA}-Dec)$ | Npts |
|---------|------------------------|------------------------|--------------------------|--------------------------|------|
| Y       | 0.00418                | 0.04464                | -0.02529                 | 0.04920                  | 352  |
| J       | 0.00915                | 0.05083                | -0.03439                 | 0.06893                  | 485  |
| H       | -0.00212               | 0.05518                | -0.00942                 | 0.06055                  | 362  |
| K       | -0.00323               | 0.05333                | -0.00660                 | 0.05896                  | 373  |
| All HSC | 0.01183                | 0.01599                | -0.01952                 | 0.02057                  | 1706 |

## 4. HSC DATA

The Archival HSC images used in Paper1 were downloaded in early 2020 from the National Astronomical Observatory of Japan SMOKA archive and were processed by co-I Kikuta using the HSC pipeline (Bosch et al. 2018), which removes instrumental signatures of individual images, calibrates the astrometry and photometry using Pan-STARRS (Tonry et al. 2012) and creates stacked images in the different observed bands. As described in Paper1, a cutout of  $\sim 30.80' \times 33.59'$  centered at (17:22:48.1298, +65:50:14.853, J2000) was selected from the HEROES NEP-wide-A05 field at 17:26:31.206 +65:31:57.98 J2000.0, which covered all of the ancillary data available in early 2020. Figure 5 shows the distribution of astrometric offsets between the HSC and GAIA DR3 positions and the mean values are shown in the bottom row of Table 1.

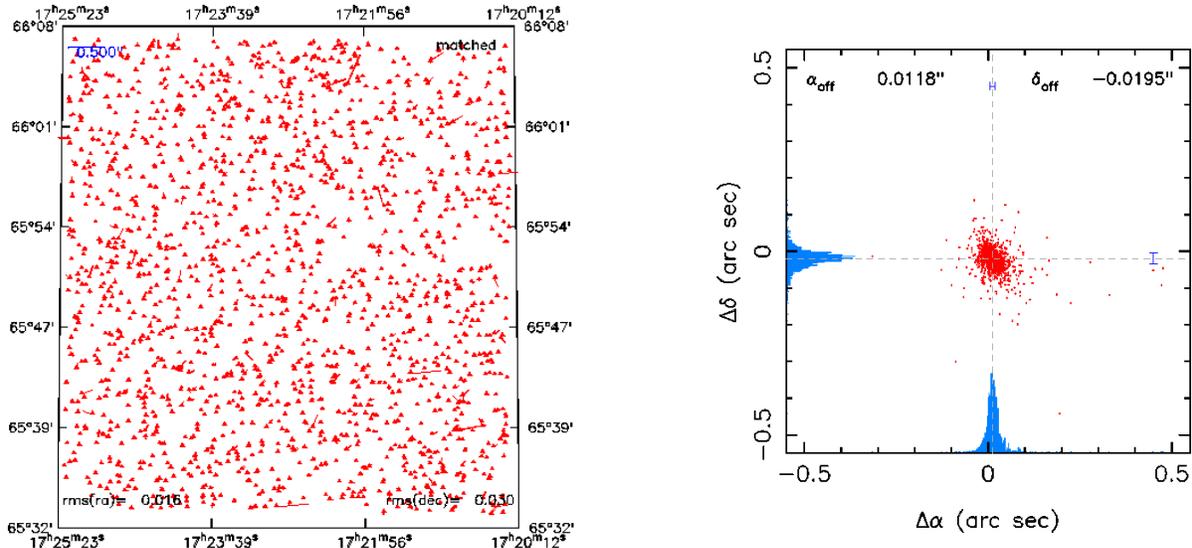

**Figure 5.** Same as in Figure 1, but for the HSC mosaics. In contrast to the MMIRS imaging where catalogues were constructed from single mosaics, the HSC catalogues are derived from dual-mode **SExtractor** detections, using a  $\chi^2$  image (Szalay et al. 1999), and there are no differences in the positions measured in the HSC wide bands.

With the publication of the HEROES survey catalogue by Taylor et al. (2023), we carried out an assessment of our NEP TDF HSC **SExtractor** photometry. The NEP TDF is covered by three HEROES pointings, one of them new, specifically targeting the NEP TDF (Taylor et al. 2023). Figure 7 shows the exposures added. The Taylor et al. (2023) catalogues include results from additional images obtained from 2021 onwards in the *z* and *NB921* filters, besides new sets of data using the *r2* and *HSC-Y* filters as shown in Figure 7.

As described by Taylor et al. (2023), the HEROES catalog subdivides the survey into several patches, which have some overlap, and the observations reduced as part of PEARLS are covered by four patches— **17,9**, **17,10**, **18,9** and **18,10** as shown in Figure 6. As described in Paper1, we used the catalogue of unique sources (**HEROES\_Full\_Catalog.fits**) to recover some of the photometric measurements only available in the patch-level catalogues. Restricting the area to that covered by the PEARLS HSC NEP TDF we have a total of 150,216 sources selected after applying the position limits of  $260.0583 \leq \text{R.A.} \leq 261.3350$  and  $65.550 \leq \text{Dec.} \leq 66.125$ , and, following Taylor et al. (2023), using the flags

$$\text{is\_primary} = 1, \quad (1)$$

and for each filter

$$\{g,i2,z,NB816,NB921\}\_base\_PixelFlags\_flag\_edge = false, \quad (2)$$

and

$$\{g,i2,z,NB816,NB921\}\_base\_PixelFlags\_bad = false \quad (3)$$

to select a sample of sources that are not blended and that are not contaminated by the proximity to very bright neighbours and diffraction spikes. Matching the HEROES sub-catalogue with PEARLS HSC produces a list of 55,796 common sources. As described in Paper1, we selected stellar sources to compare the photometry, and following [Bosch et al. \(2018\)](#), used the distribution of HEROES MAG\_PSF magnitudes versus the MAG\_PSF – MAG\_CMODEL magnitude difference. In the comparison that follows, we restricted sources to having

$$\| \text{MAG\_PSF} - \text{MAG\_CMODEL} \| \leq 0.01 \quad (4)$$

for all wide band filters and only considering sources with  $17.5 \leq i2 \leq 23.5$ . The measurements allow recovering the stellar locus, traced by the  $r2-i2$  versus  $g-r2$  colour differences for 2219 stars displayed in Figure 8.

The HSC pipeline ([Bosch et al. 2018](#)), produces aperture-corrected values for the total magnitudes, whereas our measurements are not aperture-corrected. To compare our measurements with the HEROES magnitudes, we used the [Taylor et al. \(2023\)](#) aperture magnitudes calculated at a radius of 12 pixels, corresponding to a **SExtractor** aperture diameter of  $4''.03$ . This aperture is large enough to contain the bulk of the light while being less affected by noise. Figures 9 through 13 show the magnitude differences versus HEROES magnitudes and histograms of the magnitude differences for the 5 filters in common, using the stellar sources of Figure 8; Table 2 reproduces the values presented in Table 7 of Paper1 and shows the offsets in magnitudes and errors and the multiplier used to convert the fluxes of PEARLS sources.

The right panel of these figures shows the magnitude differences as histogrammes and shows the IDL `resistant_mean` values for the average difference and dispersion. For the  $g$  and  $z$  bands the differences are small, while an offset is clearly seen for the  $i2$  filter, the PEARLS **SExtractor** magnitudes being brighter. The differences measured in the

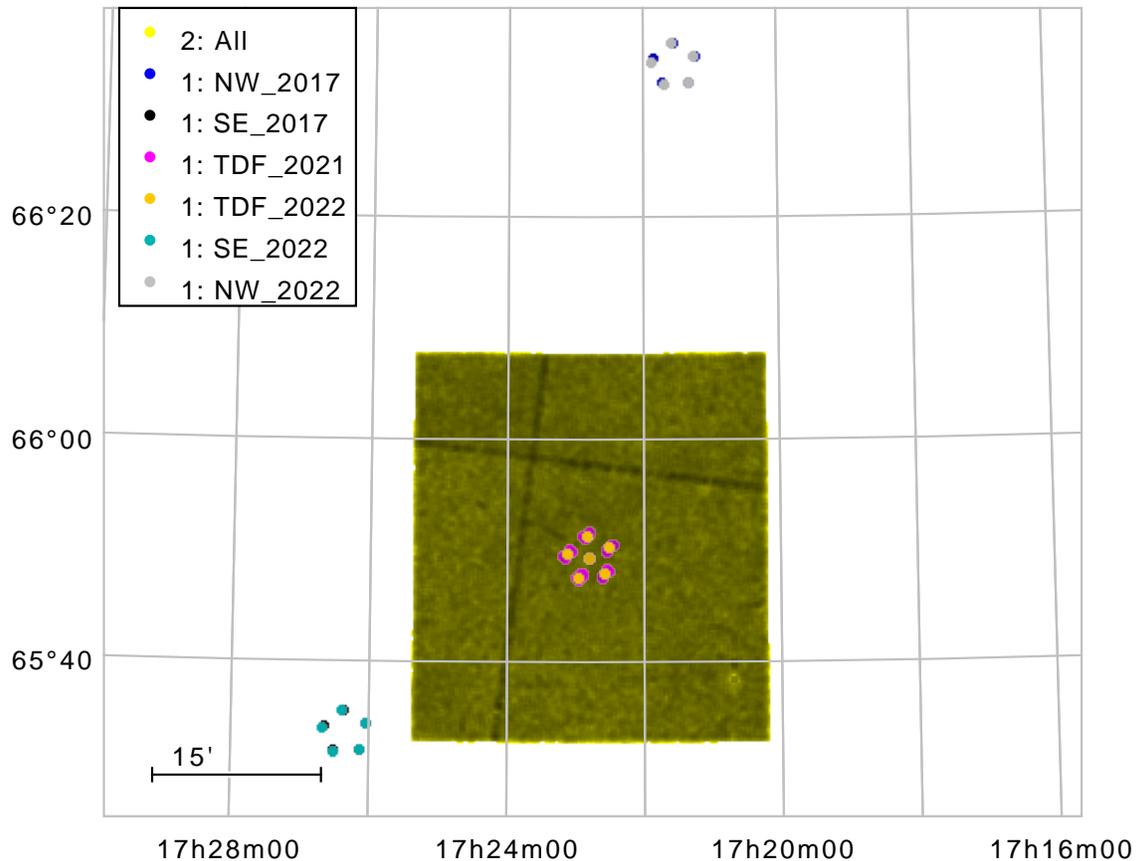

**Figure 6.** Projected distribution of [Taylor et al. \(2023\)](#) sources in the NEP TDF region (grey points). The coloured circles indicate the HSC pointing centres and the years these were observed as noted in the key. The darker stripes show the regions where the patches overlap; these duplicate sources are removed in the final full-field catalogue of [Taylor et al. \(2023\)](#). The PEARLS HSC catalogue is derived from measurements obtained in the SE.2017 pointing (*NEP-wide-A05*) at 17:26:31.206 +65:31:57.98 J2000.0

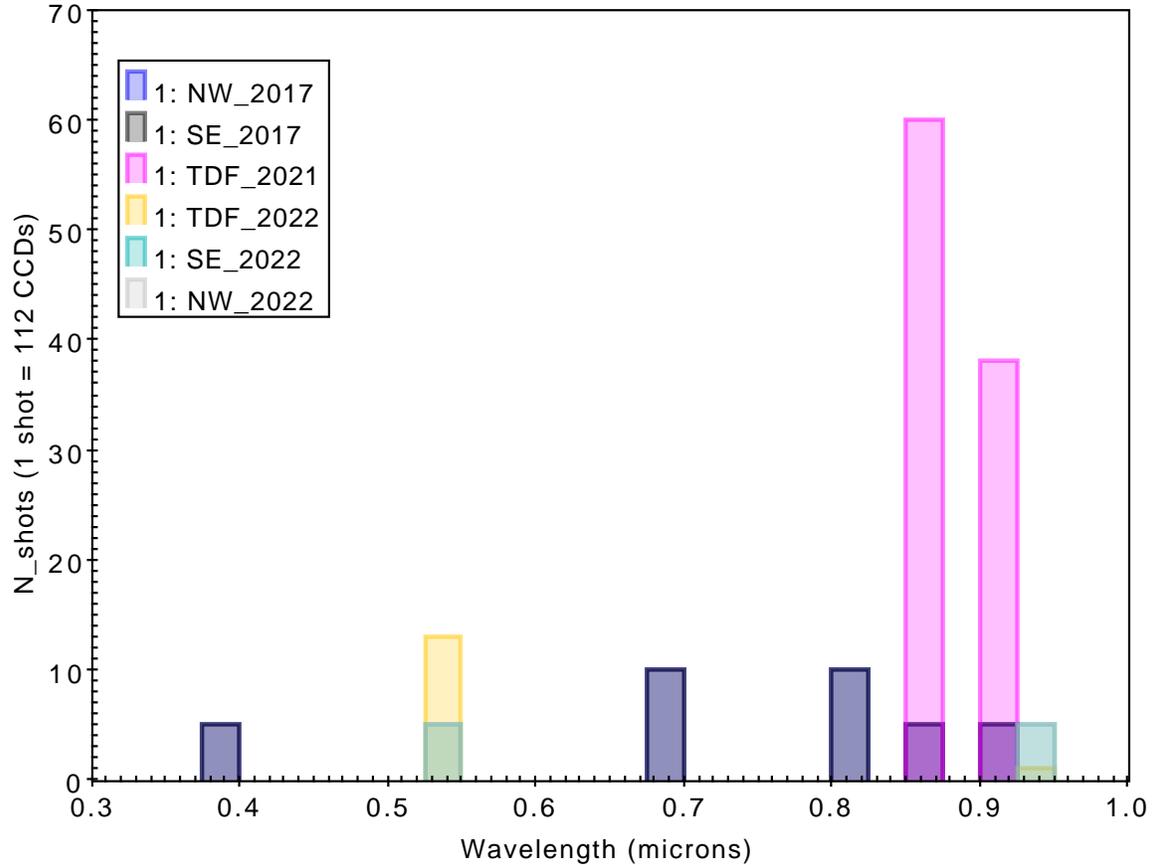

**Figure 7.** Histogram showing the number of exposures per filter in the general TDF area where different colours denote different epochs of observation. As noted in Figure 6, the NEP contains data from 3 different locations, one of them specifically centred on the NEP TDF (Taylor et al. 2023). The latter comprise observations in  $r2$  (yellow bar at  $0.54 \mu\text{m}$ ),  $z$ , and  $NB921$  (pink bars at  $0.86 \mu\text{m}$  and  $0.92 \mu\text{m}$  respectively).

narrow-band filters are negligible. The final HSC-MMIRS merged catalogue uses these offsets to correct all magnitudes and fluxes. The effect of these corrections in the wide-band filters can be seen in Figure 14, which plots the stellar locus using the original `SExtractor` measurements in grey, the HEROES values in blue and the corrected `SExtractor` as orange points, which now overlap the HEROES data.

**Table 2.** Magnitude differences between HEROES HSC and PEARLS `SExtractor` measurements (.

| Filter  | $N_{stars}$ | mean difference | uncertainty | Flux correction |
|---------|-------------|-----------------|-------------|-----------------|
| $g$     | 2219        | -0.022          | 0.052       | 1.02043         |
| $i2$    | 2219        | +0.087          | 0.025       | 0.92318         |
| $z$     | 2219        | -0.012          | 0.025       | 1.01125         |
| $NB816$ | 2219        | -0.009          | 0.033       | 1.00789         |
| $NB921$ | 2219        | -0.009          | 0.030       | 1.00790         |

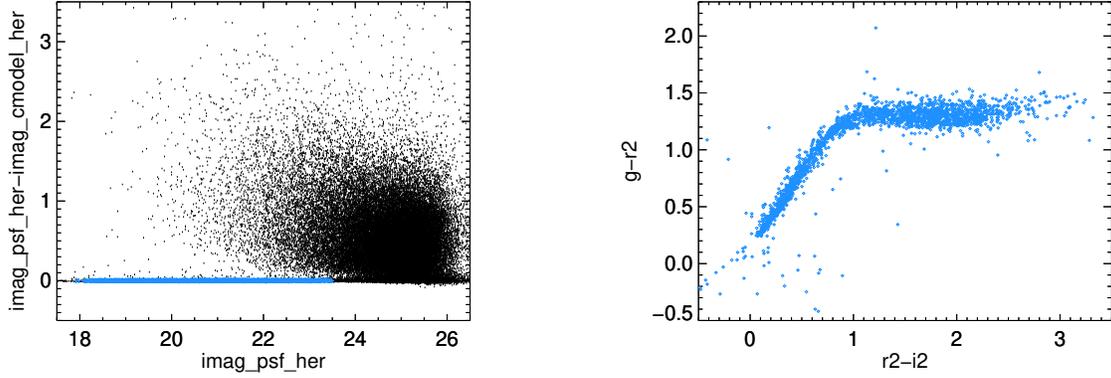

**Figure 8.** Left panel: selection of stars using the difference between the `MAG_PSF` and `MAG_CMODEL` magnitudes, following Bosch et al. (2018). The objects selected as stars fall on the small magnitude difference ridge and were selected as such only if they fell on this ridge in all wide band HSC filters. Right panel: the stellar locus derived from the magnitude differences.

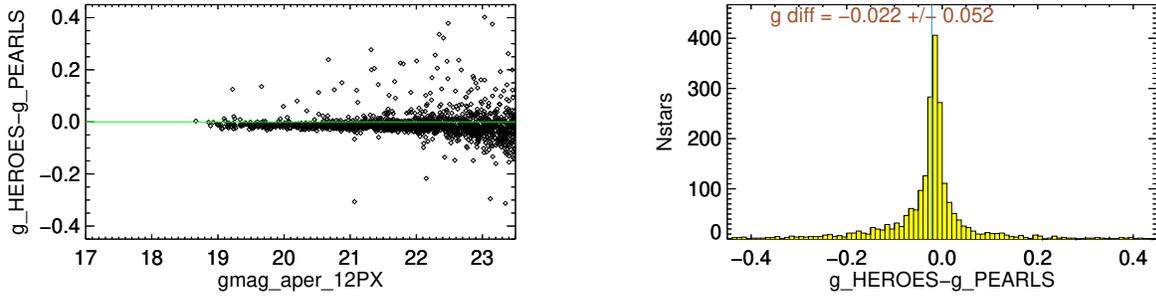

**Figure 9.** Left panel: Distribution of aperture magnitudes as measured by the HSC pipeline (Bosch et al. 2018) from Taylor et al. (2023) and the magnitude difference relative to the PEARLS `SExtractor` `mag_aper` values in the HSC *g* band. In this comparison we use the HEROES aperture of 12 pixels *radius*, which corresponds to a  $4''.03$  *diameter* aperture. The horizontal green line represents magnitude differences of 0. Right panel: histogramme of the magnitude differences with the IDL `resistant_mean` average and dispersion values.

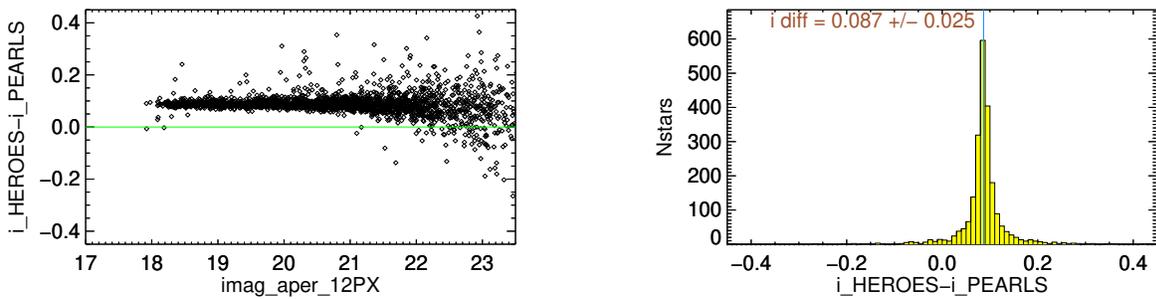

**Figure 10.** Comparison between aperture magnitudes as in Figure 9 for the *i2* band measurements.

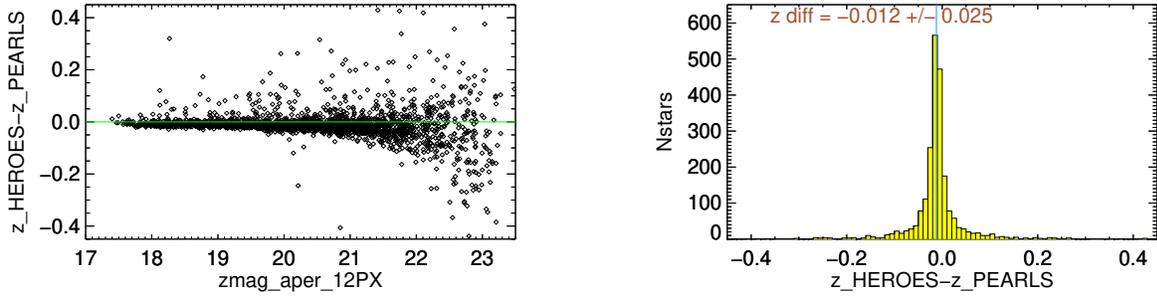

**Figure 11.** Comparison between aperture magnitudes as in Figure 9 for z band measurements.

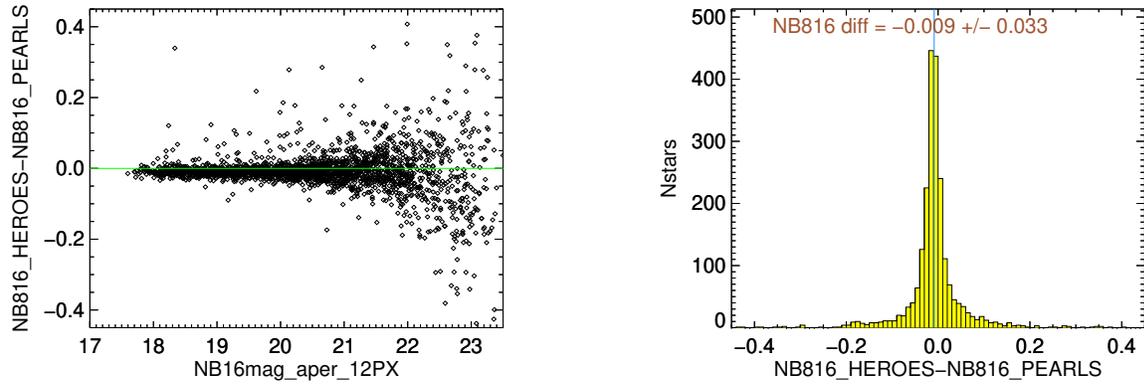

**Figure 12.** Comparison between aperture magnitudes as in Figure 9 for the NB816 band measurements.

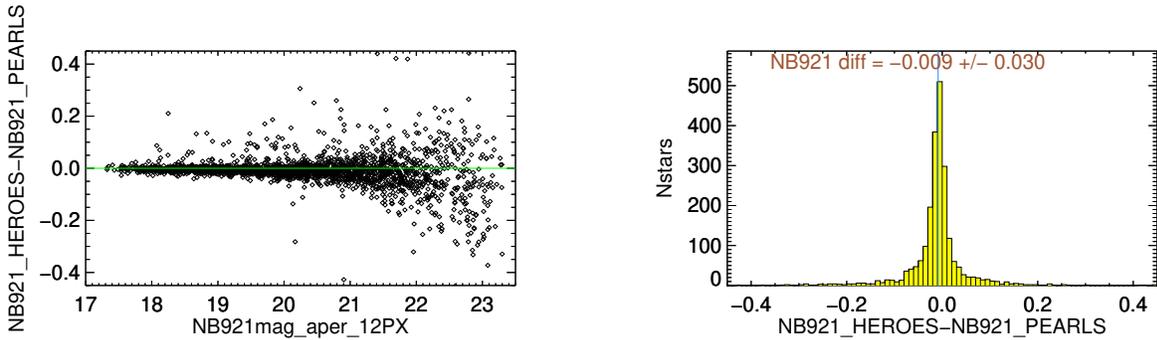

**Figure 13.** Comparison between aperture magnitudes as in Figure 9 for the NB921 band measurements.

Even though MMIRS and HEROES both contain Y filters, we decided not to compare these measurements as the throughput shapes, shown in Figure 15 are significantly different that colour terms would be required to make a meaningful comparison.

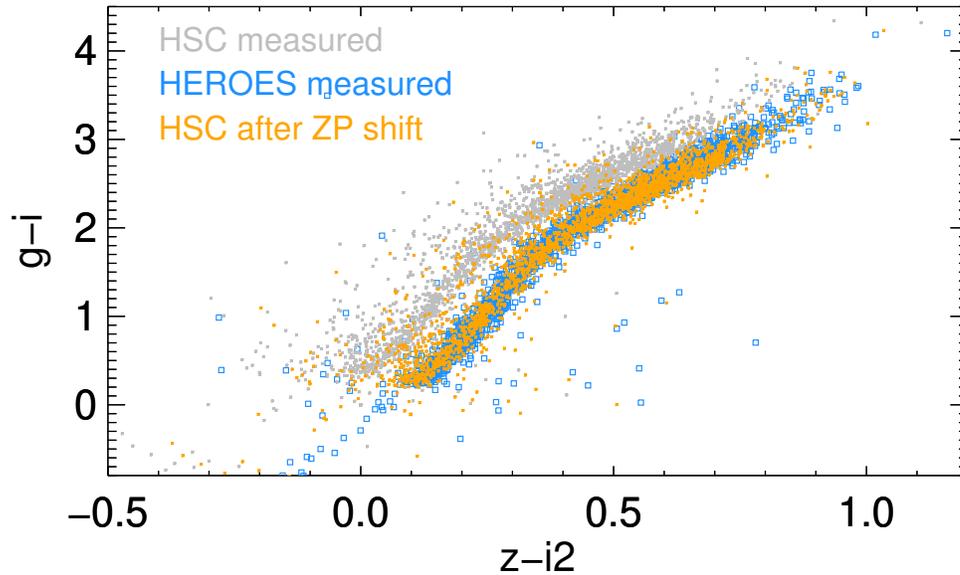

**Figure 14.** Stellar locus of HEROES and HSC measurements. The grey points are calculated from `SExtractor` `MAG_PSF` measurements, and are shifted relative to the HEROES stellar locus. Once the offsets are added, both sets of measurements show good agreement.

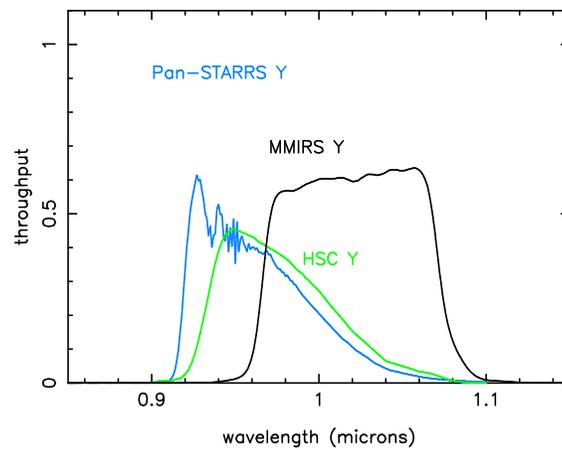

**Figure 15.** Comparison between the Y throughput profiles of Pan-STARRS (blue), HSC (green) and MMIRS (black). In all cases the profiles contain the contribution due to the filter, detector and telescope. The MMIRS filter covers longer wavelengths than both the Pan-STARRS and HSC filters.

#### 4.1. Limiting magnitudes

The estimated completeness using single band detections (i.e., without the use of the  $\chi^2$  image) is shown in Figure 16. The calculation followed the same procedure as Paper1, using Monte-Carlo simulations where 100 sources are added at random positions in the image in 100 simulations for each magnitude bin of 0.1 magnitudes. The vertical lines denote the completeness levels for 95%, 80% and 50% recovery rates; these values are presented in Table 3.

**Table 3.** Completeness levels for HSC filters.

| Filter       | $m_{AB}(95\%)$ | $m_{AB}(80\%)$ | $m_{AB}(50\%)$ | minarea | threshold |
|--------------|----------------|----------------|----------------|---------|-----------|
| <i>g</i>     | 25.68          | 26.05          | 26.27          | 10      | 1.1       |
| <i>i2</i>    | 24.50          | 24.87          | 25.18          | 10      | 1.1       |
| <i>z</i>     | 24.09          | 24.36          | 24.60          | 10      | 1.1       |
| <i>NB816</i> | 23.96          | 24.17          | 24.43          | 10      | 1.1       |
| <i>NB921</i> | 24.08          | 24.28          | 24.51          | 10      | 1.1       |

#### 4.2. Number counts

The number counts for galaxies in the PEARLS NEP TDF HSC imaging are presented as black circles in Figure 17. We also include number counts using the sub-catalogue derived from Taylor et al. (2023), restricted to the NEP TDF footprint showing counts for the combined extended+compact sources (blue open crosses), compact objects (grey stars) and extended ones (brown solid boxes). Also shown are published counts in the wide band filters by Davies et al. (2021) (orange asterisks) of galaxies using a combination of several ground-based catalogues, and the total source counts by Taylor et al. (2023) which contain compact+extended sources for magnitudes measured within a  $2''$  diameter aperture for the entire HEROES field as well as similar counts from the HSC-COSMOS survey (blue points) and the Dark Energy Survey Year 3 results (Green points). The agreement between the number counts for PEARLS and the NEP TDF HEROES sub-catalogue and those in Davies et al. (2021) is very good. The total number counts (compact+extended sources) for the NEP TDF HEROES sub-catalogue agrees well with the Taylor et al. (2023). At brighter magnitudes ( $i2 \lesssim 18.5$ ) the galaxy counts for the NEP TDF are lower than the Davies et al. (2021) values, which is a combination small number statistics and uncertain star/galaxy separation at magnitudes where stars become saturated and have significant diffraction spikes. Because the catalogues are derived using dual-mode detection with a stacked  $\chi^2$  image, the magnitude limits attained by the different band is slightly fainter than those measured from the completeness simulations described above.

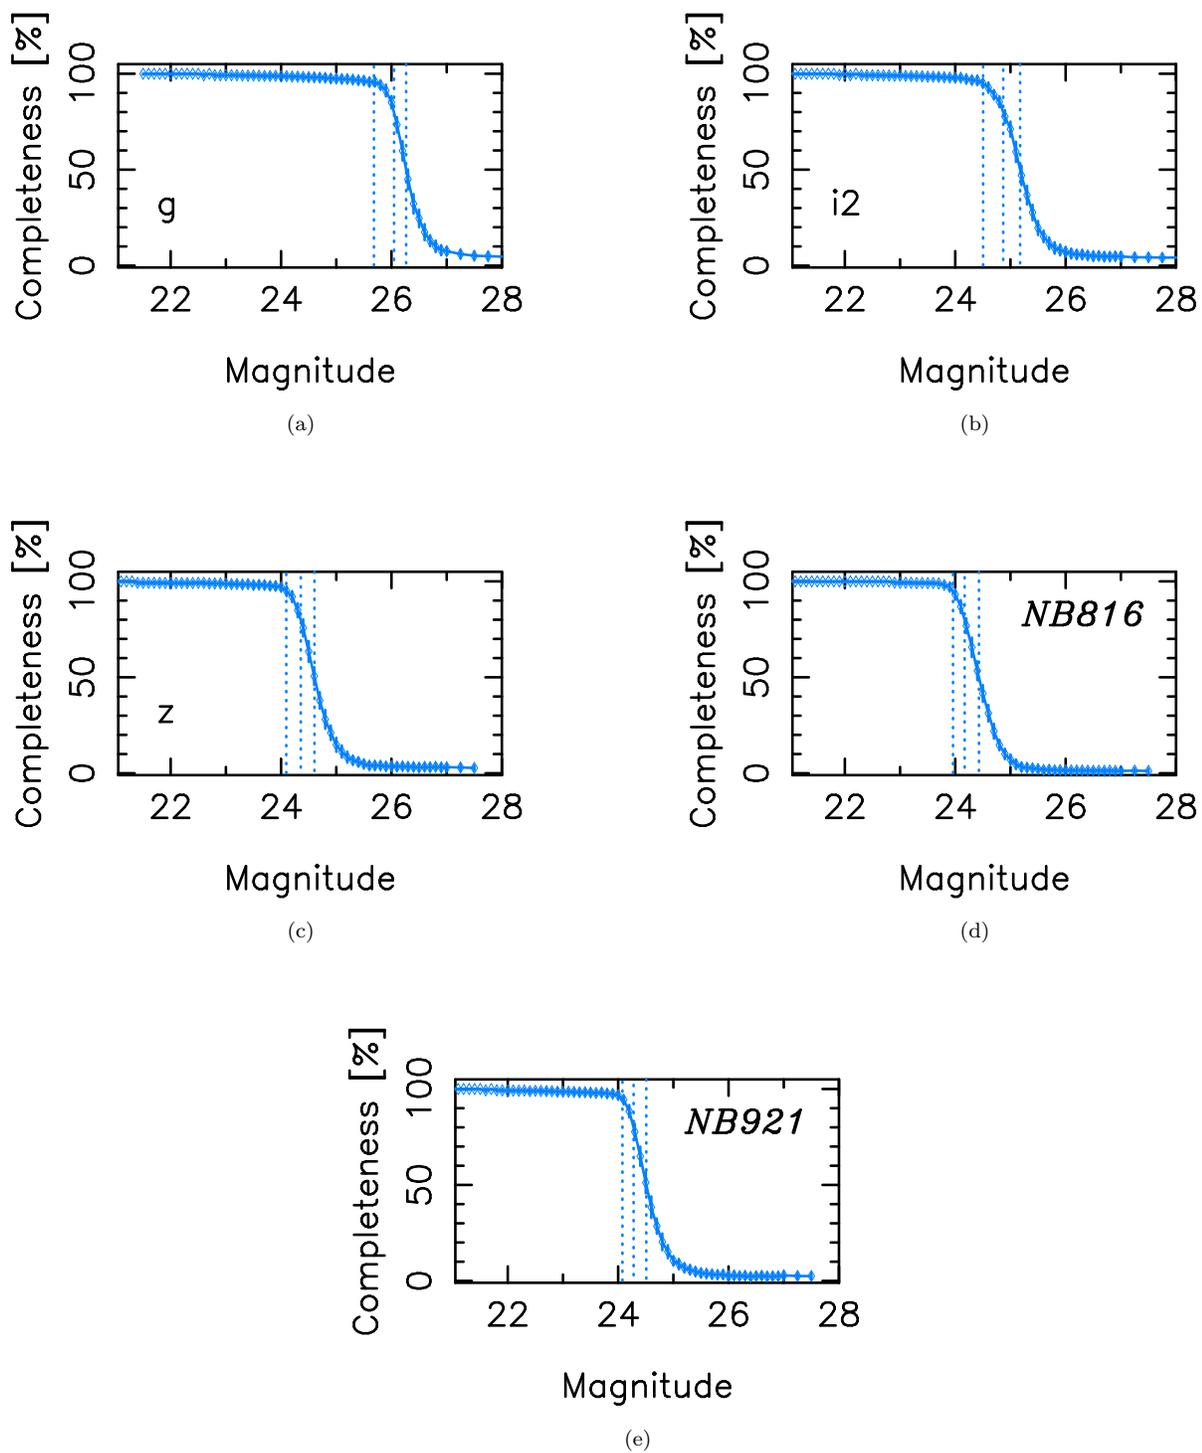

**Figure 16.** Completeness levels for the HSC bands for point sources using Monte Carlo simulations in single band detections. The vertical lines indicate (from left to right) the 95%, 80%, and 50% completeness levels.

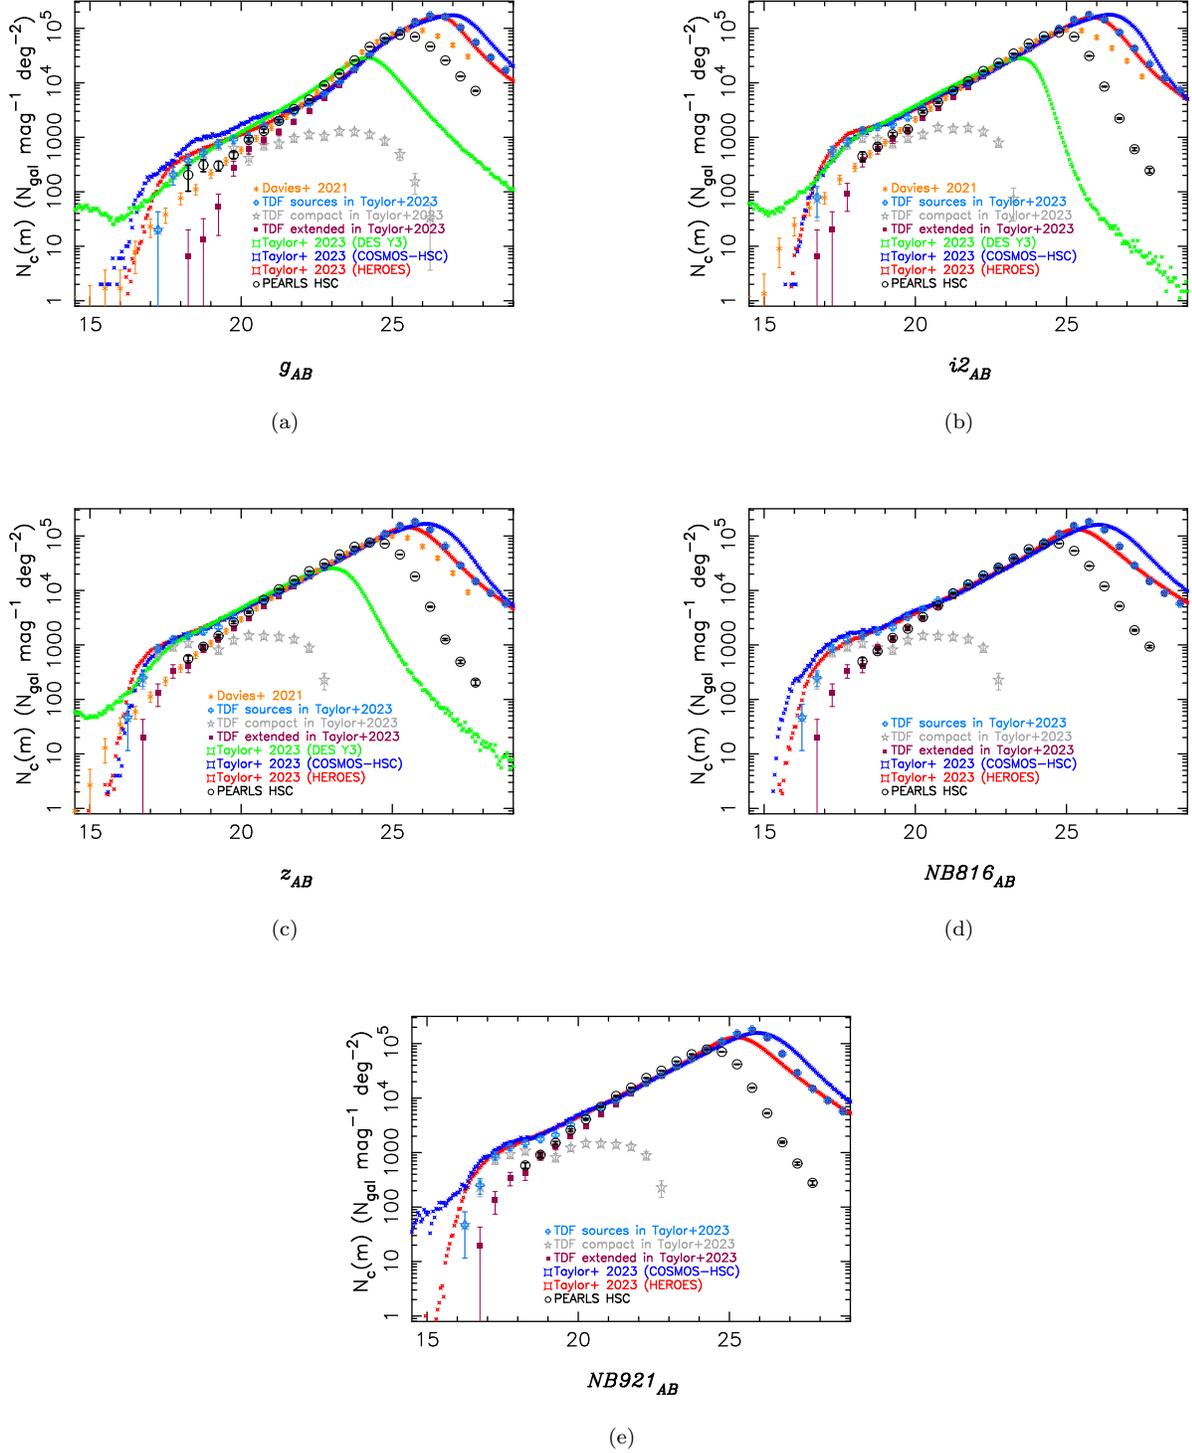

**Figure 17.** Differential galaxy number counts ( $N_c(m)$ ) measured for the PEARLS HSC catalogue (black open circles), counts for compact (grey stars), extended (brown solid squares) and the combined compact+extended sources (blue crosses) for the NEP TDF region using a sub-catalogue derived from Taylor et al. (2023). Also shown are galaxy counts by Davies et al. (2021) in the wide-band filters, and measurements made by Taylor et al. (2023) using stars and galaxies in the full HEROES catalogue (red points), the HSC-COSMOS survey (dark blue points) and the Dark Energy Survey Year 3 sample (Sevilla-Noarbe et al. 2021; Hartley et al. 2022). The PEARLS HSC counts use the SExtractor MAG\_AUTO parameter while aperture magnitudes within  $2''$  were used for data derived from the HEROES catalogue. At magnitudes fainter than 22 the agreement between all surveys is good. The decrease in the number of galaxies for magnitudes of 18 and brighter the TDF sub-catalogue is a combination of uncertain star/galaxy separation and small number statistics.

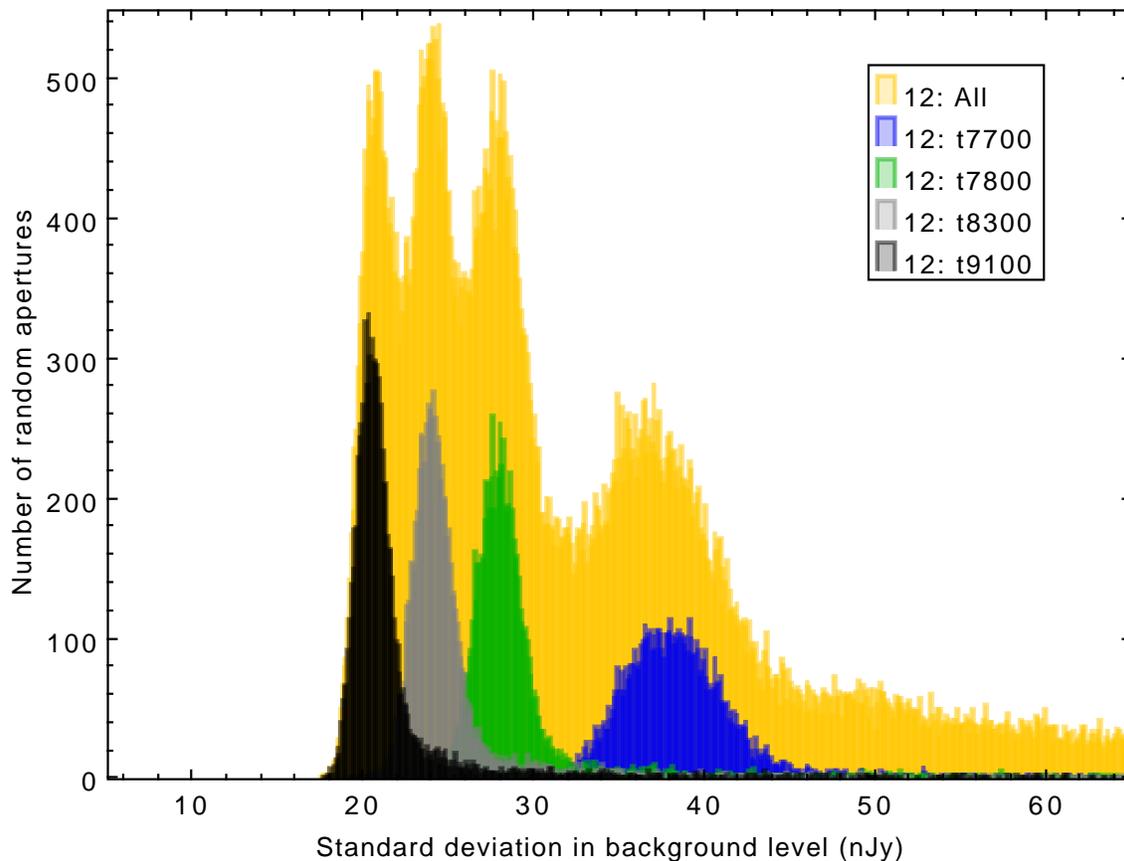

**Figure 18.** Distribution of number of random apertures at a given standard deviation of the background level for the combine  $K+K_{\text{spec}}$  mosaic. The different coloured peaks represent locations on the image where the total exposure times are  $\sim 9,100$  s (black, leftmost peak),  $\sim 8300$  s (grey, second peak from left to right),  $\sim 7800$  s (green, third peak) and  $\sim 7700$  s (blue, fourth peak). The last peak is from the region in the image covered by the  $K_{0.95}$  and  $K_{\text{spec}}$  imaging, both of which have higher Poisson noise levels, compared to the default  $K_{2.68}$  imaging.

## 5. KNOWN ISSUES

As shown in Section 3, the NIR imaging still presents some distortions which are not completely removed when calculating the astrometric solutions. Other issues in the MMIRS mosaics are non-uniformities in the background, affecting the  $K+K_{\text{spec}}$  mosaic and is particularly noted in the SE quadrant of the field which is covered by the wider  $K_{\text{spec}}$  and the higher gain  $K_{0.95}$  imaging, as shown in Figure 18. The Y image also shows short-scale variations in the background.

## 6. RELEASE CONTENT

This data release comprises FITS table catalogues and FITS image mosaics from the HSC and MMIRS imaging in the NEP TDF, which are made available in Zenodo under an open-source Creative Commons Attribution license: [doi:10.5281/zenodo.7934393](https://doi.org/10.5281/zenodo.7934393).

The files are listed in Table 4 and include the matched catalogue of sources containing HSC and MMIRS detections and a catalogue of spurious sources due to image defects and diffraction spikes of bright stars. The parameters contained by these catalogues are identified in Table 5. We include a table with the measured sky conditions for each MMIRS image, which lists the number of stars being used, the seeing FWHM (noted as “biwt” in the FITS table), the airmass, and sky level counts and dispersion. We should note that the FWHM, elongation and ellipticity are bi-weight averages (Beers et al. 1990) from measurements of all detected stars. Finally, we add the table containing a sub-set of HEROES measurements of sources within the NEP TDF, used in Section 4 of this document. The image mosaics are

**Table 4.** Files on zenodo.

| file type                   | file name                                        |
|-----------------------------|--------------------------------------------------|
| This document               | NEP_MMIRS_HSC_data_release.pdf                   |
| Catalog sources             | hsc_mmirs_clean_2023_07_12.fits                  |
| Catalog of spurious sources | hsc_mmirs_junk_2023_07_12.fits                   |
| Seeing measurements         | mmirs_psf_psfex_2023_05_20.fits                  |
| HEROES sub-catalog in TDF   | heroes_forced_tdf_2023_06_01.fits                |
| science image               | NEP_HSC_G.fits                                   |
| science image               | NEP_HSC_I.fits                                   |
| science image               | NEP_HSC_Z.fits                                   |
| science image               | NEP_HSC_NB816.fits                               |
| science image               | NEP_HSC_NB921.fits                               |
| science image               | NEP_H_mosaic_sci_2022_03_30_08_57_46.fits        |
| weight                      | NEP_H_mosaic_wht_2022_03_30_08_57_46.fits        |
| flag                        | NEP_H_mosaic_flag_2022_03_30_08_57_46.fits       |
| exposure map                | NEP_H_mosaic_exp_2.1_2022_06_12.fits             |
| science image               | NEP_J_mosaic_sci_2022_04_07_21_49_33.fits        |
| weight                      | NEP_J_mosaic_wht_2022_04_07_21_49_33.fits        |
| flag                        | NEP_J_mosaic_flag_2022_04_07_21_49_33.fits       |
| exposure map                | NEP_J_mosaic_exp_2.1_2022_06_12.fits             |
| science image               | NEP_K_0.95_mosaic_sci_2022_03_31_05_47_10.fits   |
| weight                      | NEP_K_0.95_mosaic_wht_2022_03_31_05_47_10.fits   |
| flag                        | NEP_K_0.95_mosaic_flag_2022_03_31_05_47_10.fits  |
| exposure map                | NEP_K_0.95_mosaic_exp_2.1_2022_06_12.fits        |
| science image               | NEP_K_2.68_mosaic_sci_2022_03_31_12_56_40.fits   |
| weight                      | NEP_K_2.68_mosaic_wht_2022_03_31_12_56_40.fits   |
| flag                        | NEP_K_2.68_mosaic_flag_2022_03_31_12_56_40.fits  |
| exposure map                | NEP_K_2.68_mosaic_exp_2.1_2022_06_12.fits        |
| science image               | NEP_Kspec_mosaic_sci_2022_03_31_22_06_59.fits    |
| weight                      | NEP_Kspec_mosaic_wht_2022_03_31_22_06_59.fits    |
| flag                        | NEP_Kspec_mosaic_flag_2022_03_31_22_06_59.fits   |
| exposure map                | NEP_Kspec_mosaic_exp_2.1_2022_06_12.fits         |
| science image               | NEP_K+Kspec_mosaic_sci_2022_04_01_14_13_20.fits  |
| weight                      | NEP_K+Kspec_mosaic_wht_2022_04_01_14_13_20.fits  |
| flag                        | NEP_K+Kspec_mosaic_flag_2022_04_01_14_13_20.fits |
| exposure map                | NEP_K+Kspec_mosaic_exp_2.1_2022_06_11.fits       |
| science image               | NEP_Y_mosaic_sci_2022_03_30_04_11_37.fits        |
| weight                      | NEP_Y_mosaic_wht_2022_03_30_04_11_37.fits        |
| flag                        | NEP_Y_mosaic_flag_2022_03_30_04_11_37.fits       |
| exposure map                | NEP_Y_mosaic_exp_2.1_2022_06_12.fits             |

derived from the new MMIRS observations we carried out and, in the case of HSC data, from archival raw data that were publicly available in the SMOKA archive in early 2020. For MMIRS images, we provide the science mosaics, the weight images calculated by `swarp`, flag images derived from the weight images to denote pixels without valid data, and exposure maps. In the case of HSC data, we only provide the science images that come from the reduction using the HSC pipeline of [Bosch et al. \(2018\)](#).

**Table 5.** Catalogue parameters.

| Column         | Description                                                                  |
|----------------|------------------------------------------------------------------------------|
| UNIQUE_ID      | Object’s unique identification                                               |
| OBJID          | HSC object ID                                                                |
| RA             | Right Ascension for equinox J2000                                            |
| DEC            | Declination for equinox J2000                                                |
| ALPHAWIN_J2000 | Windowed Right Ascension for equinox J2000                                   |
| DELTAWIN_J2000 | Windowed Declination for equinox J2000                                       |
| THETA_J2000    | Position angle of semi-major axis from N to E                                |
| ELLIPTICITY    | Ellipticity calculated by <i>SExtractor</i>                                  |
| ELONGATION     | Object elongation calculate by <i>SExtractor</i>                             |
| A_WORLD        | Semi-major axis in arcseconds                                                |
| ERRA_WORLD     | Semi-major axis in arcseconds                                                |
| B_WORLD        | Semi-minor axis in arcseconds                                                |
| ERRB_WORLD     | Semi-minor axis in arcseconds                                                |
| X_IMAGE        | x pixel coordinate of source’s barycenter                                    |
| Y_IMAGE        | y pixel coordinate of source’s barycenter                                    |
| XMIN_IMAGE     | minimum X position for the object’s segmentation map                         |
| YMIN_IMAGE     | minimum Y position for the object’s segmentation map                         |
| XMAX_IMAGE     | maximum X position for the object’s segmentation map                         |
| YMAX_IMAGE     | maximum Y position for the object’s segmentation map                         |
| XPEAK_IMAGE    | X position for the object’s brightest pixel                                  |
| YPEAK_IMAGE    | Y position for the object’s brightest pixel                                  |
| GCLASS_STAR    | Object classification using <i>SExtractor</i> ’s neural network <sup>a</sup> |
| GFLAGS         | <i>SExtractor</i> detection flags                                            |
| GRKRON         | Kron radius in arcsec                                                        |
| GPETRO_RADIUS  | Petrosian radius in arcsec                                                   |
| GFLUX_RADIUS   | Half-light radius in arcsec                                                  |
| GFWHM_ARCSEC   | FWHM of point-sources in arcsec                                              |
| GISOAREAF      | Area in squared pixels contained by the limiting isophote                    |
| GISOAREA       | Area in squared pixels contained by the limiting isophote                    |
| GFLUX_MAX      | Flux in the brightest pixel                                                  |
| GMU_MAX        | Surface brightness of the brightest pixel                                    |
| GMU_THRESHOLD  | Surface brightness at detection threshold                                    |
| GBACKGROUND    | Background level at source position                                          |
| GMAG_PETRO     | Petrosian magnitude (AB)                                                     |
| GMAGERR_PETRO  | Petrosian magnitude error (AB)                                               |
| GFLUX_PETRO    | Petrosian flux (nJy)                                                         |
| GFLUXERR_PETRO | Petrosian flux error (nJy)                                                   |
| GMAG_AUTO      | ”Total” magnitude calculated within Kron radius                              |

**Table 5** continued on next page

Table 5 (continued)

| Column           | Description                                                               |
|------------------|---------------------------------------------------------------------------|
| GMAGERR_AUTO     | "Total" magnitude error calculated within Kron radius                     |
| GFLUX_AUTO       | "Total" flux calculated within Kron radius (nJy)                          |
| GFLUXERR_AUTO    | "Total" flux error calculated within Kron radius (nJy)                    |
| GMAG_PSF         | PSF magnitude integrated over best-fitting PSF model (AB)                 |
| GMAGERR_PSF      | PSF magnitude error of best-fitting PSF model (AB)                        |
| GFLUX_PSF        | PSF flux integrated over best-fitting PSF model (nJy)                     |
| GFLUXERR_PSF     | PSF flux error of best-fitting PSF model (nJy)                            |
| GMAG_APER_020    | Magnitude integrated over a 0.2" diameter circular aperture <sup>b</sup>  |
| GMAGERR_APER_020 | Magnitude error of 0.2" diameter circular aperture <sup>b</sup>           |
| GMAG_APER_050    | Magnitude integrated over a 0.5" diameter circular aperture <sup>b</sup>  |
| GMAGERR_APER_050 | Magnitude error of 0.5" diameter circular aperture <sup>b</sup>           |
| GMAG_APER_068    | Magnitude integrated over a 0.68" diameter circular aperture <sup>b</sup> |
| GMAGERR_APER_068 | Magnitude error of 0.68" diameter circular aperture <sup>b</sup>          |
| GMAG_APER_080    | Magnitude integrated over a 0.8" diameter circular aperture <sup>b</sup>  |
| GMAGERR_APER_080 | Magnitude error of 0.8" diameter circular aperture <sup>b</sup>           |
| GMAG_APER_100    | Magnitude integrated over a 1.0" diameter circular aperture <sup>b</sup>  |
| GMAGERR_APER_100 | Magnitude error of 1.0" diameter circular aperture <sup>b</sup>           |
| GMAG_APER_120    | Magnitude integrated over a 1.2" diameter circular aperture <sup>b</sup>  |
| GMAGERR_APER_120 | Magnitude error of 1.2" diameter circular aperture <sup>b</sup>           |
| GMAG_APER_136    | Magnitude integrated over a 1.36" diameter circular aperture <sup>b</sup> |
| GMAGERR_APER_136 | Magnitude error of 1.36" diameter circular aperture <sup>b</sup>          |
| GMAG_APER_150    | Magnitude integrated over a 1.5" diameter circular aperture <sup>b</sup>  |
| GMAGERR_APER_150 | Magnitude error of 1.5" diameter circular aperture <sup>b</sup>           |
| GMAG_APER_180    | Magnitude integrated over a 1.8" diameter circular aperture <sup>b</sup>  |
| GMAGERR_APER_180 | Magnitude error of 1.8" diameter circular aperture <sup>b</sup>           |
| GMAG_APER_200    | Magnitude integrated over a 2.0" diameter circular aperture <sup>b</sup>  |
| GMAGERR_APER_200 | Magnitude error of 2.0" diameter circular aperture <sup>b</sup>           |
| GMAG_APER_250    | Magnitude integrated over a 2.5" diameter circular aperture <sup>b</sup>  |
| GMAGERR_APER_250 | Magnitude error of 2.5" diameter circular aperture <sup>b</sup>           |
| GMAG_APER_300    | Magnitude integrated over a 3.0" diameter circular aperture <sup>b</sup>  |
| GMAGERR_APER_300 | Magnitude error of 3.0" diameter circular aperture <sup>b</sup>           |
| GMAG_APER_350    | Magnitude integrated over a 3.5" diameter circular aperture <sup>b</sup>  |
| GMAGERR_APER_350 | Magnitude error of 3.5" diameter circular aperture <sup>b</sup>           |
| GMAG_APER_400    | Magnitude integrated over a 4.0" diameter circular aperture <sup>b</sup>  |
| GMAGERR_APER_400 | Magnitude error of 4.0" diameter circular aperture <sup>b</sup>           |
| GMAG_APER_500    | Magnitude integrated over a 5.0" diameter circular aperture <sup>b</sup>  |
| GMAGERR_APER_500 | Magnitude error of 5.0" diameter circular aperture <sup>b</sup>           |
| GMAG_APER_600    | Magnitude integrated over a 6.0" diameter circular aperture <sup>b</sup>  |
| GMAGERR_APER_600 | Magnitude error of 6.0" diameter circular aperture <sup>b</sup>           |

<sup>a</sup>These parameters follow the same nomenclature for different filters, where the prefix will be G, I, Z, NB816, NB921, H, J, K and Y.

<sup>b</sup>The aperture values in arcsec are found by dividing the numerical value by 100; for the NIR filters we also tabulate the corresponding fluxes and errors in nJy.

## 7. CONCLUSION

This document described in more detail some of the characteristics of the visible-near infrared images we make available in the NEP TDF, combining archival observations of the Subaru Hyper-Suprime-Cam and new observations of with MMIRS on the MMT. The astrometric calibration shows a dispersion  $\leq 20$  mas for HSC and  $\leq 70$  mas for the MMIRS imaging, with negligible zero-point offsets relative to Gaia. The HSC offsets are consistent with a random distribution, while those from MMIRS show systematic deviations up to  $\sim 15$  mas with the presence of a few poles, though the cause is unclear. We also compare our HSC photometry with measurements published by Taylor et al. (2023) for the HEROES survey. We find offsets of  $\sim +0.087$  magnitudes for the *HSC-i2* filter, where our PEARLS measurements are brighter, and offsets ranging from  $-0.022$  to  $-0.009$  magnitudes for the remaining filters. Reaching depths of  $\sim 25.7$  (*g*) and  $24.1$  (*z*), these data were essential to calibrate astrometrically the JWST NEP TDF observations of GTO proposal 2738 (PI: Windhorst & Hammel) and provide a reference for future studies of variability within this field.

## 8. ACKNOWLEDGEMENTS

We thank our late colleague Mario Nonino for suggesting us to write this document. We thank Anthony Taylor for providing the table of HEROES number counts and for insight on the HSC pipeline reduction, and Catherine Grier for providing the script that calculates exposure maps using `swarp`. We respectfully acknowledge that the University of Arizona and Arizona State University are on the land and territories of Indigenous peoples. Today, Arizona is home to 22 federally recognized tribes, with Tucson being home to the O’odham and the Yaqui and Tempe home to the Akimel O’odham (Pima) and Pee Posh (Maricopa). We wish to recognize and acknowledge the very significant cultural role and reverence that the summit of Mauna Kea has always had within the Kānaka Maoli community. We are most fortunate to have the opportunity of using observations obtained on this mountain. CNAW acknowledges support from the NIRCcam Development Contract NAS5-02105 from NASA Goddard Space Flight Center to the University of Arizona. CNAW and RAJ gratefully acknowledge funding from the HST-GO-15278.008-A grant. RAW, SHC, and RAJ acknowledge support from NASA JWST Interdisciplinary Scientist grants NAG5-12460, NNX14AN10G and 80NSSC18K0200 from GSFC. We acknowledge the SMOKA archive of the National Astronomical Observatory of Japan from which Subaru *Hyper-Suprime-Cam* data were retrieved. This work has made use of data from the European Space Agency (ESA) mission *Gaia* (<https://www.cosmos.esa.int/gaia>), processed by the *Gaia* Data Processing and Analysis Consortium (DPAC, <https://www.cosmos.esa.int/web/gaia/dpac/consortium>). Funding for the DPAC has been provided by national institutions, in particular the institutions participating in the *Gaia* Multilateral Agreement.

## REFERENCES

- Abdurro’uf, Accetta, K., Aerts, C., et al. 2022, ApJS, 259, 35. doi:10.3847/1538-4365/ac4414
- Aihara, H., AIsayyad, Y., Ando, M., et al. 2022, PASJ, 74, 247. doi:10.1093/pasj/psab122
- Almeida-Fernandes, F., SamPedro, L., Herpich, F. R., et al. 2022, MNRAS, 511, 4590. doi:10.1093/mnras/stac284
- Barrett, P., Hunter, J., Miller, J. T., et al. 2005, Astronomical Data Analysis Software and Systems XIV, 347, 91
- Beers, T. C., Flynn, K., & Gebhardt, K. 1990, AJ, 100, 32
- Bertin, E. 2006, Astronomical Data Analysis Software and Systems XV, 351, 112
- Bertin, E. 2010, Astrophysics Source Code Library, ascl:1010.068
- Bertin, E., & Arnouts, S. 1996, A&AS, 117, 393
- Bertin, E., Mellier, Y., Radovich, M., et al. 2002, Astronomical Data Analysis Software and Systems XI, 281, 228
- Bertin, E. 2011, Astronomical Data Analysis Software and Systems XX, 442, 435
- Bessell, M. & Murphy, S. 2012, PASP, 124, 140. doi:10.1086/664083
- Bosch, J., Armstrong, R., Bickerton, S., et al. 2018, PASJ, 70, S5. doi:10.1093/pasj/psx080
- Caldwell, N. 2006, ApJ, 651, 822
- J., et al. 2016, MNRAS, 462, 501
- Chilingarian, I., Beletsky, Y., Moran, S., et al. 2015, PASP, 127, 406
- Coelho, P. R. T. 2014, MNRAS, 440, 1027. doi:10.1093/mnras/stu365
- Davies, L. J. M., Thorne, J. E., Robotham, A. S. G., et al. 2021, MNRAS, 506, 256. doi:10.1093/mnras/stab1601
- Eisenhardt, P., Dickinson, M., Stanford, S.A., & Ward, J.K., 2001, <https://github.com/iraf-community/iraf-xdmsum>
- Finkelstein, S. L., Ryan, R. E., Papovich, C., et al. 2015, ApJ, 810, 71. doi:10.1088/0004-637X/810/1/71

- Gaia Collaboration, Brown, A. G. A., Vallenari, A., et al. 2016, *A&A*, 595, A2. doi:10.1051/0004-6361/201629512
- Gaia Collaboration, Prusti, T., de Bruijne, J. H. J., et al. 2016, *A&A*, 595, A1
- Gaia Collaboration, Brown, A. G. A., Vallenari, A., et al. 2018, *A&A*, 616, A1
- Gaia Collaboration, Vallenari, A., Brown, A. G. A., et al. 2022, arXiv:2208.00211
- Hartley, W. G., Choi, A., Amon, A., et al. 2022, *MNRAS*, 509, 3547. doi:10.1093/mnras/stab3055
- Jansen, R. A., & Windhorst, R. A. 2018, *PASP* 130, 124001. doi:10.1088/1538-3873/aae476
- Joye, W. 2011, *Astronomical Data Analysis Software and Systems XX*, 442, 633
- Koushan, S., Driver, S. P., Bellstedt, S., et al. 2021, *MNRAS*, 503, 2033. doi:10.1093/mnras/stab540
- Labbé, I., Franx, M., Rudnick, G., et al. 2003, *AJ*, 125, 1107
- Lang, D., Hogg, D. W., Mierle, K., Blanton, M., & Roweis, S. 2010, *AJ*, 139, 1782
- McCracken, H. J., Milvang-Jensen, B., Dunlop, J., et al. 2012, *A&A*, 544, A156
- McLeod, B., Fabricant, D., Nystrom, G., et al. 2012, *PASP*, 124, 1318
- Oke, J. B. & Gunn, J. E. 1983, *ApJ*, 266, 713. doi:10.1086/160817
- Pelló, R., Hudelot, P., Laporte, N., et al. 2018, *A&A*, 620, A51. doi:10.1051/0004-6361/201732080
- Rowe, B. T. P., Jarvis, M., Mandelbaum, R., et al. 2015, *Astronomy and Computing*, 10, 121. doi:10.1016/j.ascom.2015.02.002
- Sevilla-Noarbe, I., Bechtol, K., Carrasco Kind, M., et al. 2021, *ApJS*, 254, 24. doi:10.3847/1538-4365/abeb66
- Skrutskie, M. F., Cutri, R. M., Stiening, R., et al. 2003, *IPAC*, <https://catcopy.ipac.caltech.edu/doi/doi.php?id=10.26131/IRSA2>. doi:10.26131/IRSA2
- Skrutskie, M. F., Cutri, R. M., Stiening, R., et al. 2006, *AJ*, 131, 1163. doi:10.1086/498708
- Songaila, A., Hu, E. M., Barger, A. J., et al. 2018, *ApJ*, 859, 91. doi:10.3847/1538-4357/aac021
- Szalay, A. S., Connolly, A. J., & Szokoly, G. P. 1999, *AJ*, 117, 68. doi:10.1086/300689
- Taylor, A. J., Barger, A. J., Cowie, L. L., et al. 2023, *ApJS*, 266, 24. doi:10.3847/1538-4365/accd70
- Taylor, M. B. 2005, *Astronomical Data Analysis Software and Systems XIV*, 347, 29
- Tonry, J. L., Stubbs, C. W., Lykke, K. R., et al. 2012, *ApJ*, 750, 99. doi:10.1088/0004-637X/750/2/99
- Willmer, C. N. A. 2018, *ApJS*, 236, 47. doi:10.3847/1538-4365/aabfdf
- Willmer, C. N. A., Ly, C., Kikuta, S., et al. 2023, *ApJS*, accepted.
- Windhorst, R. A., Cohen, S. H., Jansen, R. A., et al. 2023, *AJ*, 165, 13. doi:10.3847/1538-3881/aca163
